# Supplementary material for: Optical properties of CsCu$_2$X$_3$ (X=Cl, Br and I): A comparative study between hybrid time-dependent density-functional theory and the Bethe-Salpeter equation
Source: arXiv:2007.13711 ancillary file (2020-09-03)
Supplement: Supplementary file 1 [file supplemental.pdf]

# Supplemental material for: Optical properties of $CsCu_2X_3$ (X=Cl, Br and I): A comparative study between hybrid time-dependent density-functional theory and the Bethe-Salpeter equation

Jiuyu Sun and Carsten A. Ullrich
*Department of Physics and Astronomy, University of Missouri, Columbia, Missouri 65211, USA*
(Dated: September 1, 2020)

## I. LDA AND PBE BAND STRUCTURES AND THE ROLE OF PSEUDOPOTENTIALS

In the present work, we adopted norm-conserving pseudopotentials (PSPs) in both the Quantum Espresso [1] and the Yambo code [2]. In principle, we should use the optimized norm-conserving Vanderbilt pseudopotentials (ONCVPSPs) [3, 4], a library of well generated and tested PSPs, for all the elements considered in this work. However, the ONCVPSP of Cs corresponding to the LDA functional is not provided. Instead, we used the Troullier-Martins [5] PSP for Cs, which is available on the official website of Quantum Espresso [6]. Although these two types of PSPs are both norm-conserving, a validation of mixing them should be performed.

Since we considered the experimental structures for all three $CsCu_2X_3$, there is no need to check the geometry structures obtained by the mixed PSPs. Thus we compare the electronic structures obtained by LDA with mixed PSPs and PBE with all ONCVPSPs. In Fig. 1, we plot the band structures for $CsCu_2Cl_3$. It is obvious that the valence band parts are almost identical to each other. Except for a downward shift due to the slightly smaller band gap (see Table 1 in the main paper), the LDA conduction band part is also very close to that obtained with PBE. This confirms that the mixed PSPs can be safely used for $CsCu_2X_3$.

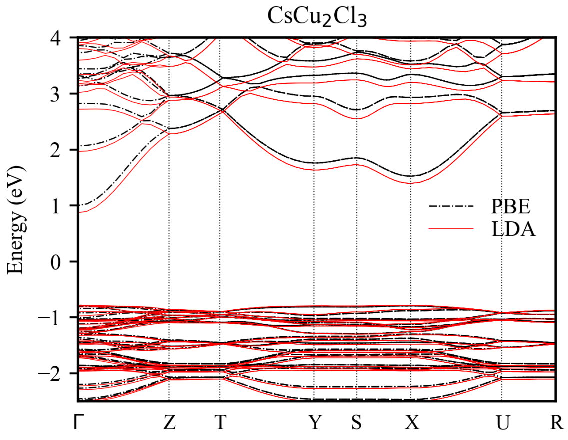


FIG. 1. Band structure of $CsCu_2Cl_3$, obtained with LDA using mixed PSPs and with PBE using only ONCVPSPs.

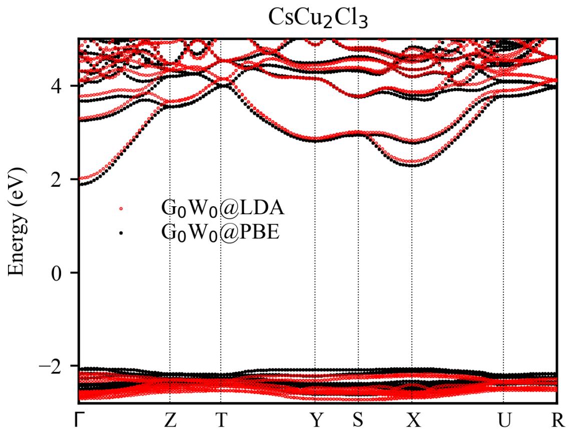


FIG. 2. Band structure of $CsCu_2Cl_3$, obtained with $G_0W_0$@LDA and $G_0W_0$@PBE.

## II. COMPARISON OF $G_0W_0$@LDA AND $G_0W_0$@PBE BAND STRUCTURES

In Fig. 2, we plot the band structures of $CsCu_2Cl_3$, obtained with $G_0W_0$@LDA and $G_0W_0$@PBE. Ignoring the slightly different band gaps (see Table 1 in the main paper), the $G_0W_0$@LDA and $G_0W_0$@PBE valence band parts are almost identical. For the conduction bands, the parts from 2 eV to 4 eV are also quite close. However, the parts above 4 eV exhibit some differences around the U point.

In this work, we focus on the low-lying optical excitations at or below the band gap ($E_g^{QP} = 4.2$ eV for $CsCu_2Cl_3$, see Table 1 in the main paper), which arise mainly from a coherent superposition of the quasiparticle excitations near the band edges. As seen from the band structures in Fig. 2, the lowest-energy quasi-electron-hole pairs will be located around the Γ and X points. The slight differences between the $G_0W_0$@LDA and $G_0W_0$@PBE bands above 4 eV around the U point have practically no influence on the low-lying optical excitations. Thus, we choose the $G_0W_0$@LDA band structures to correct the DFT bands in the calculations of the optical properties of $CsCu_2X_3$.

TABLE I. Band gaps of $CsCu_2X_3$, calculated with DFT, hybrid functionals and $G_0W_0$, and RPA inverse dielectric constant $1/\varepsilon_0$ along [111]. All hybrid functionals are evaluated using the single-shot approach, except PBEsc from Ref. [7]. All energies are in eV.

| | $CsCu_2Cl_3$ | $CsCu_2Br_3$ | $CsCu_2I_3$ |
|---|---|---|---|
| LDA | 1.65 | 1.40 | 1.79 |
| LDA0 | 4.70 | 4.16 | 3.75 |
| DDH1@LDA | 5.84 | 4.67 | 3.79 |
| DDH2@LDA | 5.59 | 4.47 | 4.13 |
| $G_0W_0$@LDA | 4.20 | 3.63 | 4.03 |
| $G_0W_0$@DDH2 | 4.85 | 4.17 | 4.53 |
| COHSEX | 4.69 | 4.01 | 4.31 |
| $1/\varepsilon_0$ | 0.343 | 0.296 | 0.245 |
| | | | |
| PBE | 1.78 | 1.59 | 1.98 |
| PBE0 | 4.48 | 3.96 | 4.04 |
| PBE0sc (from Ref. [7]) | 4.29 | 3.88 | 3.93 |
| DDH1@PBE | 5.25 | 4.27 | 3.95 |
| DDH2@PBE | 5.20 | 4.24 | 3.93 |
| $G_0W_0$@PBE | 3.92 | 3.47 | 3.83 |
| $1/\varepsilon_0$ | 0.318 | 0.280 | 0.239 |

## III. BAND GAPS BY SINGLE-SHOT HYBRID FUNCTIONALS AND $G_0W_0$

In the main paper, we noted that the calculated quasiparticle gap of $CsCu_2Br_3$ is smaller than in $CsCu_2Cl_3$ and $CsCu_2I_3$, whereas the exciton binding energies and dielectric constants suggest a different trend for the gap. In this section we explore the performance of the various types of hybrid functionals discussed in the main paper for calculating fundamental band gaps. We consider single-shot global hybrid functionals using the ground states from LDA (LDA0, DDH1@LDA, DDH2@LDA) and PBE (PBE0, DDH1@PBE, DDH2@PBE) as input. All calculated band gaps are listed in Table I.

In typical implementations of hybrid functionals, the generalized Kohn-Sham equation (featuring a nonlocal exchange potential) is solved self-consistently. By contrast, in the single-shot approach, we first obtain the self-consistent LDA or PBE ground state, use the resulting Kohn-Sham orbitals as input to construct the hybrid functional, and then solve the generalized Kohn-Sham equation once more, without further iteration. Clearly, this is computationally cheaper than a fully self-consistent implementation, which is why we use it here.

We first consider the LDA0 and PBE0 band gaps, where the admixture of exact exchange ($a = 0.25$) is material-independent. Among the three materials, the LDA0 and PBE0 band gaps of $CsCu_2Cl_3$ have the largest increase over the LDA and PBE gaps, respectively. Thus, the nonlocal Fock exchange has the greatest effect in $CsCu_2Cl_3$. However, LDA0 and PBE0 yield different trends: in LDA0, the gap shrinks from X=Cl to I, whereas in PBE0, the gap shrinks from Cl to Br, but increases from Br to I. One also finds that the single-shot PBE0 is in quite close agreement to the self-consistent PBE0sc in Ref. [7]. The PBE0 gaps are a bit overestimated (by 0.1-0.2 eV) compared to PBE0sc.

Owing to the larger prefactors of Fock exchange (i.e., more screening), all the DDHs result in larger band gaps than LDA0 and PBE0 for $CsCu_2Cl_3$ and $CsCu_2Br_3$. When the inverse dielectric constants ($1/\varepsilon_0$) are close to 0.25, the band gaps of $CsCu_2I_3$ produced by all the hybrid functionals, as well as $G_0W_0$, become very similar to each other. The band gaps decrease from $CsCu_2Cl_3$ to $CsCu_2I_3$ for all DDHs, which is not observed for $G_0W_0$: the $G_0W_0$ gap for X=I is larger than the gap for X=Br.

In refs. [8, 9] it was noted that that perovskites are very sensitive to the $G_0W_0$ starting point, and LDA or PBE are often insufficient. This suggests to try a DDH hybrid functional as starting point. A fully self-consistent calculation of the DDH band structure is beyond the scope of this work; instead, we used the band gaps by single-shot DDH2 and applied scissor shifts to LDA energies as input for $G_0W_0$; we refer to this approach as $G_0W_0$@DDH2. Table I shows that for $CsCu_2Br_3$, the band gap by $G_0W_0$@DDH2 is 4.17 eV, which is significantly enlarged compared to the gap by $G_0W_0$@LDA. However, the trend problem still persists with $G_0W_0$@DDH2. Table I also lists the band gaps by COHSEX, which can be regarded as a simplified $G_0W_0$ and which is closely related to the DDHs (see main paper). The band gap of $CsCu_2Br_3$ by COHSEX is still smaller than those in other two materials, although the difference between $CsCu_2Br_3$ and $CsCu_2I_3$ is now less pronounced.

Overall, Table I shows that the DDH gaps are consistently larger than the $G_0W_0$ gaps (with the exception of $CsCu_2I_3$). The DDH1 and DDH2 gaps are very close to each other. Clearly, only the hybrid functionals are capable of producing the (presumably) correct trend of the band gaps of the copper halides. However, to completely settle this issue, in particular with respect to the starting point dependence of $G_0W_0$, further study is required.

Lastly, we compare the experimental optical gaps $E_g^{opt}$ (see Table II of the main paper), with those obtained by combining the DDH hybrid band gaps and exciton binding energies $E_b$, see Table III in the main paper, and with the corresponding results using the $G_0W_0$ band gaps and the BSE. Generally, the DDH+DDH (single-shot DDH band gaps plus DDH exciton binding energies) optical gaps are significantly larger than the $G_0W_0$+BSE optical gaps. For $CsCu_2Br_3$ we find $E_g^{opt} = 3.9$ eV (using the DDH2@PBE gap), which agrees much better with experiment than BSE. On the other hand, for $CsCu_2Cl_3$ we find $E_g^{opt} = 4.5$ eV (again using the DDH2@PBE gap), which is worse than BSE. For $CsCu_2I_3$, all methods agree rather closely with each other.

Thus, based on these results it is not possible to conclude that DDH+DDH produces better optical gaps than $G_0W_0$+BSE. It remains to be seen whether a self-consistent implementation of the DDH band structure or more advanced many-body approaches (as discussed in the main text) lead to improvements.

TABLE II. $G_0W_0$@LDA band gaps ($E_{\text{gap}}^{GW}$) obtained by using different number of bands $N_{\text{bands}}$, and DFT energy levels ($E^{\text{DFT}}$) of the corresponding highest band. All energies are in eV.

| $N_{\text{bands}}$ | 400 | | 450 | | 500 | |
|---|---|---|---|---|---|---|
| | $E_{\text{gap}}^{GW}$ | $E^{\text{DFT}}$ | $E_{\text{gap}}^{GW}$ | $E^{\text{DFT}}$ | $E_{\text{gap}}^{GW}$ | $E^{\text{DFT}}$ |
| $CsCu_2Cl_3$ | 4.20 | 30.30 | 4.23 | 33.86 | 4.19 | 36.68 |
| $CsCu_2Br_3$ | 3.63 | 24.97 | 3.62 | 28.61 | 3.61 | 31.89 |
| $CsCu_2I_3$ | 4.03 | 24.73 | 4.02 | 28.26 | 4.01 | 31.21 |

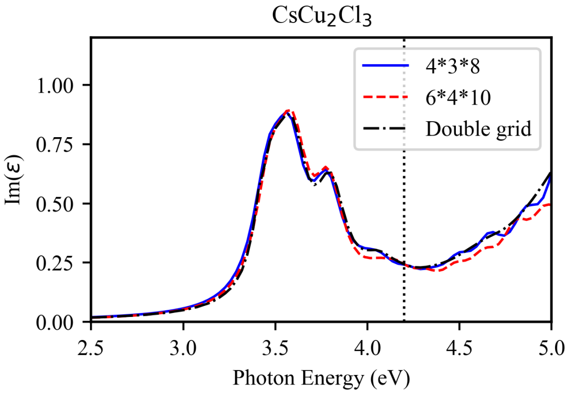


FIG. 3. $G_0W_0$+BSE optical spectra Im($\varepsilon$) calculated with different **k**-grids. The vertical dotted lines indicate the positions of the $G_0W_0$@LDA band gaps.

## IV. CONVERGENCE TESTS

We tested the convergence behavior of the $G_0W_0$@LDA band gap as a function of the number of bands ($N_{\text{bands}}$) included in the calculation; the results are shown in Table II. We also list the DFT energy levels ($E^{\text{DFT}}$) of the corresponding highest band involved. As $N_{\text{bands}}$ increases from 400 to 500, the changes of the band gaps are minimal, which clearly shows that the calculations are sufficiently converged using $N_{\text{bands}} = 400$.

To test the convergence depending on the **k**-grid, we compare results obtained using two Γ centered meshes, Mesh1 (4×3×8, used in the paper) and Mesh2 (6×4×10). The calculated $G_0W_0$@LDA band gap of $CsCu_2Cl_3$ with Mesh2 is 4.21 eV, which is very close to the gap of 4.20 eV obtained with Mesh1. In addition, the inverse dielectric constant $\varepsilon^{-1}$ by Mesh2 is 0.3428, which is the same as $\varepsilon^{-1}$ by Mesh1 to within 4 digits.

Using the quasiparticle energy correction obtained with Mesh2, we also performed a BSE calculation for $CsCu_2Cl_3$. The optical spectra are plotted in Fig. 3. The red and blue lines are obtained with the Γ-centered uniform **k**-point meshes $4 \times 3 \times 8$ (Mesh1) and $6 \times 4 \times 10$ (Mesh2), respectively. The black line is obtained with the double grid (Mesh3) used in the main paper, consisting of a $4 \times 3 \times 8$ uniform mesh plus 3000 random interpolated **k**-points. Mesh3 can be regarded as a mesh of much higher density of **k** points. The obtained exciton binding energies are 718 meV, 710 meV and 701 meV using Mesh1, Mesh2 and Mesh3, respectively. The spread of 17 meV (i.e., 2.4%) of the exciton binding energies indicates that our calculations represent a very good compromise between sufficient numerical accuracy and affordable computational cost.

Consider now the spectra shown in Fig. 3. We first observe that three spectra are very similar to each other, except for the somewhat lower Im($\varepsilon$) beyond 4 eV for Mesh2. The reason is that the number of valence bands for Mesh2 is 45, which is smaller than 56 for Mesh1 and Mesh3, due to the limitation of computational resources. We also note that the spectrum obtained using Mesh3 is much smoother than those by Mesh1 and Mesh2, which is a consequence or the higher **k**-point density of the double grid.


[1] P Giannozzi *et al.*, Advanced capabilities for materials modelling with QUANTUM ESPRESSO, J. Phys.: Condens. Matter **29**, 465901 (2017).

[2] D. Sangalli, A. Ferretti, H. Miranda, C. Attaccalite, I. Marri, E. Cannuccia, P. Melo, M. Marsili, F. Paleari, A. Marrazzo, G. Prandini, P. Bonfà, M. O. Atambo, F. Affinito, M. Palummo, A. Molina-Sánchez, C. Hogan, M. Grning, D. Varsano, and A. Marini, Many-body perturbation theory calculations using the yambo code, J. Phys.: Condens. Matter **31**, 325902 (2019).

[3] D. R. Hamann, Optimized norm-conserving Vanderbilt pseudopotentials, Phys. Rev. B **88**, 085117 (2013), erratum: *ibid.* **95**, 239906 (2017).

[4] M. van Setten, M. Giantomassi, E. Bousquet, M. Verstraete, D. Hamann, X. Gonze, and G.-M. Rignanese, The pseudodojo: Training and grading a 85 element optimized norm-conserving pseudopotential table, Comput. Phys. Commun. **226**, 39 (2018).

[5] N. Troullier and J. L. Martins, Efficient pseudopotentials for plane-wave calculations, Phys. Rev. B **43**, 1993 (1991).

[6] https://www.quantum-espresso.org/.

[7] M.-H. Du, Emission Trend of Multiple Self-Trapped Excitons in Luminescent 1D Copper Halides, ACS Energy Lett. **5**, 464 (2020).

[8] M. R. Filip and F. Giustino, *GW* quasiparticle band gap of the hybrid organic-inorganic perovskite $CH_3NH_3PbI_3$: Ef-

fect of spin-orbit interaction, semicore electrons, and self-consistency, Phys. Rev. B **90**, 245145 (2014).

[9] L. Leppert, T. Rangel, and J. B. Neaton, Towards predictive band gaps for halide perovskites: Lessons from one-shot and eigenvalue self-consistent $GW$, Phys. Rev. Mater. **3**, 103803 (2019).
